# Supplementary material for: Text-Derived Knowledge Helps Vision: A Simple Cross-modal Distillation for Video-based Action Anticipation
Source: arXiv:2210.05991 source file (2023-02-21)
Supplement: Supplementary file 1 [file appendix.tex]

\section{Appendix}\label{sec:appendix}
In this section, we present examples of model prediction for the video action anticipation task for the \texttt{EPIC-55} dataset. For each instance we show the top-5 predictions for (i) video-only model - \textbf{\texttt{AVT}} (ii) text-based teacher model - \texttt{LM-teacher} (\textbf{\texttt{Rcp-ALBERT}}) (iii) a \texttt{LM-teacher} distilled student video model - \texttt{AVT + LM teacher Distl} (\textbf{\texttt{AVT + Rcp-ALBERT Distillation}}). Note that the end-task setting is such that, the inference has to be done only from the video frames, as the text label for the action segment won't be available during the inference time.

\par Figure~\href{fig:base_w_teacher_c_distil_c1}{3} and~4 shows example of cases where the base video only model makes incorrect prediction, where as the text-based teacher and the teacher-distilled video  model makes correct predictions.  Figure~5 and~6 shows example of cases where the base video only model makes incorrect prediction, the text-based teacher  makes correct prediction, however the teacher-distilled video  model makes incorrect predictions.
% ------------------------------------------------------------------
% Case: Base wrong, teacher correct, student correct
% EXAMPLE 1 & 2
% ------------------------------------------------------------------
\captionsetup[figure]{labelformat=empty}
\begin{figure*}[!ht]
{
  \begin{tabular}{ m{2.8cm}  m{2.8cm}  m{2.8cm}  m{2.8cm}  m{2.8cm}  }
    \hline\hline
    % ------------------------------------------------------------
    % EXAMPLE-1    
    % ------------------------------------------------------------
    \multicolumn{5}{c}{\textbf{EXAMPLE 1}} \\ \hline \hline
    \multicolumn{5}{l}{\textbf{INPUT}} \\
    \begin{minipage}{.18\textwidth}
      \includegraphics[width=\linewidth, height=30mm]{images/34base_W_teach_c_distil_c/34-5_put-down_vegetable.jpg}
      \caption{\texttt{put-down\_vegetable}}
    \end{minipage}
    &
    \begin{minipage}{.18\textwidth}
     \includegraphics[width=\linewidth, height=30mm]{images/34base_W_teach_c_distil_c/34-4_open_door.jpg}
     \caption{\texttt{open\_door}}
    \end{minipage}
    &
    \begin{minipage}{.18\textwidth}
      \includegraphics[width=\linewidth, height=30mm]{images/34base_W_teach_c_distil_c/34-3_take_greater.jpg}
      \caption{\texttt{take\_greater}}
    \end{minipage}    
    &
    \begin{minipage}{.18\textwidth}
      \includegraphics[width=\linewidth, height=30mm]{images/34base_W_teach_c_distil_c/34-2_take_pan.jpg}
    \caption{\texttt{take\_pan}}
    \end{minipage}    
    &
    \begin{minipage}{.18\textwidth}
      \includegraphics[width=\linewidth, height=30mm]{images/34base_W_teach_c_distil_c/34-1_ put-down_pan.jpg}
      \caption{\texttt{put-down\_pan}}
    \end{minipage}
    \\ \hline
    \multicolumn{5}{l}{\textbf{TARGET}: \texttt{close\_door}} \\ \hline
    \multicolumn{5}{l}{\textbf{PREDICTIONS}} \\ 
    \multicolumn{5}{l}{\texttt{\textbf{AVT} : [put-down\_pan, take\_pan, turn-on\_hob, open\_door, open\_drawer]}} \\ 
    \multicolumn{5}{l}{\texttt{\textbf{LM-teacher} : [open\_door, \textcolor{red}{close\_door}, put-down\_pan, take\_pan, turn-on\_hob]}} \\
    \multicolumn{5}{l}{\texttt{\textbf{AVT + LM teacher Distl} : [put-down\_pan, take\_pan, open\_door, \textcolor{red}{close\_door},}}\\
    \multicolumn{5}{l}{turn-on\_hob]} \\ \hline\hline
    % ------------------------------------------------------------
    % EXAMPLE-2    
    % ------------------------------------------------------------
    \multicolumn{5}{c}{\textbf{EXAMPLE 2}} \\ \hline \hline
    \multicolumn{5}{l}{\textbf{INPUT}} \\
    \begin{minipage}{.18\textwidth}
      \includegraphics[width=\linewidth, height=30mm]{images/4192base_W_teach_c_distil_c/4192-5_put-down_pan.jpg}
      \caption{\texttt{put-down\_pan}}
    \end{minipage}
    &
    \begin{minipage}{.18\textwidth}
     \includegraphics[width=\linewidth, height=30mm]{images/4192base_W_teach_c_distil_c/4192-4_put-lid.jpg}
     \caption{\texttt{put\_lid}}
    \end{minipage}
    &
    \begin{minipage}{.18\textwidth}
      \includegraphics[width=\linewidth, height=30mm]{images/4192base_W_teach_c_distil_c/4192-3_put-down_pan.jpg}
      \caption{\texttt{put-down\_pan}}
    \end{minipage}    
    &
    \begin{minipage}{.18\textwidth}
      \includegraphics[width=\linewidth, height=30mm]{images/4192base_W_teach_c_distil_c/4192-2_take_pan.jpg}
    \caption{\texttt{take\_pan}}
    \end{minipage}    
    &
    \begin{minipage}{.18\textwidth}
      \includegraphics[width=\linewidth, height=30mm]{images/4192base_W_teach_c_distil_c/4192-1_take_lid.jpg}
      \caption{\texttt{take\_lid}}
    \end{minipage}
    \\ \hline
    \multicolumn{5}{l}{\textbf{TARGET}: \texttt{put\_lid}} \\ \hline
    \multicolumn{5}{l}{\textbf{PREDICTIONS}} \\ 
    \multicolumn{5}{l}{\texttt{\textbf{AVT} : [put-down\_pan, turn-on\_hob, open\_door, take\_pan, close\_door]}} \\ 
    \multicolumn{5}{l}{\texttt{\textbf{LM-teacher}: [put-down\_pan, open\_door, take\_pan, \textcolor{red}{put\_lid}, wash\_pan]}} \\
    \multicolumn{5}{l}{\texttt{\textbf{AVT + LM teacher Distl}: [put-down\_pan, turn-on\_hob, open\_door, take\_pan, \textcolor{red}{put\_lid}]}} \\ \hline\hline    
  \end{tabular}}
  \caption{Figure 3: Example of instances where the base video-only model makes wrong prediction, whereas the text-based teacher and the teacher distilled video model makes correct prediction.}
  \label{fig:base_w_teacher_c_distil_c1}
\end{figure*}
% 
% ------------------------------------------------------------------
% Case: Base wrong, teacher correct, student correct
% EXAMPLE 3 & 4
% ------------------------------------------------------------------
\captionsetup[figure]{labelformat=empty}
\begin{figure*}[!ht]
{
  \begin{tabular}{ m{2.8cm}  m{2.8cm}  m{2.8cm}  m{2.8cm}  m{2.8cm}  }
    \hline\hline
    % ------------------------------------------------------------
    % EXAMPLE-3
    % ------------------------------------------------------------
    \multicolumn{5}{c}{\textbf{EXAMPLE 3}} \\ \hline \hline
    \multicolumn{5}{l}{\textbf{INPUT}} \\
    \begin{minipage}{.18\textwidth}
      \includegraphics[width=\linewidth, height=30mm]{images/4287base_W_teach_c_distil_c/4287-5_put-down_board-cutting.jpg}
      \caption{\texttt{put-down\_board:cutting}}
    \end{minipage}
    &
    \begin{minipage}{.18\textwidth}
     \includegraphics[width=\linewidth, height=30mm]{images/4287base_W_teach_c_distil_c/4287-4_put_onion.jpg}
     \caption{\texttt{put\_onion}}
    \end{minipage}
    &
    \begin{minipage}{.18\textwidth}
      \includegraphics[width=\linewidth, height=30mm]{images/4287base_W_teach_c_distil_c/4287-3_put_knife.jpg}
      \caption{\texttt{put\_knife}}
    \end{minipage}    
    &
    \begin{minipage}{.18\textwidth}
      \includegraphics[width=\linewidth, height=30mm]{images/4287base_W_teach_c_distil_c/4287-2_pick-up_kettle.jpg}
    \caption{\texttt{pick-up\_kettle}}
    \end{minipage}    
    &
    \begin{minipage}{.18\textwidth}
      \includegraphics[width=\linewidth, height=30mm]{images/4287base_W_teach_c_distil_c/4287-1_open_kettle.jpg}
      \caption{\texttt{open\_kettle}}
    \end{minipage}
    \\ \hline
    \multicolumn{5}{l}{\textbf{TARGET}: \texttt{fill\_kettle}} \\ \hline
    \multicolumn{5}{l}{\textbf{PREDICTIONS}} \\ 
    \multicolumn{5}{l}{\texttt{\textbf{AVT}: [open\_door, turn-on\_tap, pour\_water, close\_bin, open\_tap]}} \\ 
    \multicolumn{5}{l}{\texttt{\textbf{LM-teacher}: [pour\_water, \textcolor{red}{fill\_kettle}, put-down\_kettle, open\_kettle, close\_kettle]}} \\
    \multicolumn{5}{l}{\texttt{\textbf{AVT + LM teacher Distl}: [open\_door, pour\_water, close\_bin, \textcolor{red}{fill\_kettle},}} \\
    \multicolumn{5}{l}{turn-on\_tap]} \\ \hline\hline
    % ------------------------------------------------------------
    % EXAMPLE-  4
    % ------------------------------------------------------------
    \multicolumn{5}{c}{\textbf{EXAMPLE 4}} \\ \hline \hline
    \multicolumn{5}{l}{\textbf{INPUT}} \\
    \begin{minipage}{.19\textwidth}
      \includegraphics[width=\linewidth, height=30mm]{images/11101base_W_teach_c_distil_c/11101-5_put_lid.jpg}
      \caption{\texttt{put\_lid}}
    \end{minipage}
    &
    \begin{minipage}{.18\textwidth}
     \includegraphics[width=\linewidth, height=30mm]{images/11101base_W_teach_c_distil_c/11101-4_move_spoon.jpg}
     \caption{\texttt{move\_spoon}}
    \end{minipage}
    &
    \begin{minipage}{.18\textwidth}
      \includegraphics[width=\linewidth, height=30mm]{images/11101base_W_teach_c_distil_c/11101-3_take_flour.jpg}
      \caption{\texttt{take\_flour}}
    \end{minipage}    
    &
    \begin{minipage}{.18\textwidth}
      \includegraphics[width=\linewidth, height=30mm]{images/11101base_W_teach_c_distil_c/11101-2_open_flour.jpg}
    \caption{\texttt{open\_flour}}
    \end{minipage}    
    &
    \begin{minipage}{.18\textwidth}
      \includegraphics[width=\linewidth, height=30mm]{images/11101base_W_teach_c_distil_c/11101-1_pour_flour.jpg}
      \caption{\texttt{pour\_flour}}
    \end{minipage}
    \\ \hline
    \multicolumn{5}{l}{\textbf{TARGET}: \texttt{put-down\_flour}} \\ \hline
    \multicolumn{5}{l}{\textbf{PREDICTIONS}} \\ 
    \multicolumn{5}{l}{\texttt{\textbf{AVT} : [pour\_flour, put-down\_bag, mix\_mixture, roll\_dough, knead\_dough]}} \\ 
    \multicolumn{5}{l}{\texttt{LM-teacher : [\textcolor{red}{put-down\_flour}, pour\_flour, ' stir\_flour, mix\_mixture, check\_flour]}} \\
    \multicolumn{5}{l}{\texttt{\textbf{AVT + LM teacher Distl}: [pour\_flour, roll\_dough, mix\_mixture, put-down\_bag}} \\
    \multicolumn{5}{l}{\textcolor{red}{put-down\_flour}]} \\\hline\hline
  \end{tabular}}
  \caption{Figure 4: Example of instances where the base video-only model makes wrong prediction, whereas the text-based teacher and the teacher distilled video model makes correct prediction.} \label{fig:base_w_teacher_c_distil_c2}
\end{figure*}
% 
% ------------------------------------------------------------------
% Case: Base wrong, teacher correct, student wrong
% EXAMPLE 1 & 2
% ------------------------------------------------------------------ 
\captionsetup[table]{labelformat=empty}
\begin{figure*}[!ht]
{
  \begin{tabular}{ m{2.8cm}  m{2.8cm}  m{2.8cm}  m{2.8cm}  m{2.8cm}  }
    \hline\hline
    % ------------------------------------------------------------
    % EXAMPLE-1
    % ------------------------------------------------------------
    \multicolumn{5}{c}{\textbf{EXAMPLE 1}} \\ \hline \hline
    \multicolumn{5}{l}{\textbf{INPUT}} \\
    \begin{minipage}{.18\textwidth}
      \includegraphics[width=\linewidth, height=30mm]{images/base_w_teach_c_distil_w open_door/13-5_open_fridge.jpg}
      \caption{\texttt{open\_fridge}}
    \end{minipage}
    &
    \begin{minipage}{.18\textwidth}
     \includegraphics[width=\linewidth, height=30mm]{images/base_w_teach_c_distil_w open_door/13-4_take_carrot.jpg}
     \caption{\texttt{take\_carrot}}
    \end{minipage}
    &
    \begin{minipage}{.18\textwidth}
      \includegraphics[width=\linewidth, height=30mm]{images/base_w_teach_c_distil_w open_door/13-3_open_drawer.jpg}
      \caption{\texttt{open\_drawer}}
    \end{minipage}    
    &
    \begin{minipage}{.18\textwidth}
      \includegraphics[width=\linewidth, height=30mm]{images/base_w_teach_c_distil_w open_door/13-2_close_fridge.jpg}
    \caption{\texttt{close\_fridge}}
    \end{minipage}    
    &
    \begin{minipage}{.18\textwidth}
      \includegraphics[width=\linewidth, height=30mm]{images/base_w_teach_c_distil_w open_door/13-1_put-down_vegetable.jpg}
      \caption{\texttt{\footnotesize{putdown\_vegetable}}}
    \end{minipage}
    \\ \hline
    \multicolumn{5}{l}{\textbf{TARGET}: \texttt{open\_door}} \\ \hline
    \multicolumn{5}{l}{\textbf{PREDICTIONS}} \\ 
    \multicolumn{5}{l}{\texttt{\textbf{AVT}: [close\_door, close\_fridge, put\_container, open\_drawer, take\_knife]}} \\ 
    \multicolumn{5}{l}{\texttt{\textbf{LM-teacher}: [close\_fridge, open\_drawer, \textcolor{red}{open\_door}, close\_door, take\_sausage]
}} \\
    \multicolumn{5}{l}{\texttt{\textbf{AVT + LM teacher Distl}: [close\_door, put\_container, take\_knife, open\_drawer,}}\\
    \multicolumn{5}{l}{take\_container]} \\ \hline\hline
    % ------------------------------------------------------------
    % EXAMPLE-2 
    % ------------------------------------------------------------
    \multicolumn{5}{c}{\textbf{EXAMPLE 2}} \\ \hline \hline
    \multicolumn{5}{l}{\textbf{INPUT}} \\
    \begin{minipage}{.18\textwidth}
      \includegraphics[width=\linewidth, height=30mm]{images/base_w_teach_c_distil_w put-down_pan/4187-5_put_filter-water.jpg}
      \caption{\texttt{put\_filter:water}}
    \end{minipage}
    &
    \begin{minipage}{.18\textwidth}
     \includegraphics[width=\linewidth, height=30mm]{images/base_w_teach_c_distil_w put-down_pan/4187-4_drink-from_cup.jpg}
     \caption{\texttt{drink-from\_cup}}
    \end{minipage}
    &
    \begin{minipage}{.18\textwidth}
      \includegraphics[width=\linewidth, height=30mm]{images/base_w_teach_c_distil_w put-down_pan/4187-3_put_cup.jpg}
      \caption{\texttt{put\_cup}}
    \end{minipage}    
    &
    \begin{minipage}{.18\textwidth}
      \includegraphics[width=\linewidth, height=30mm]{images/base_w_teach_c_distil_w put-down_pan/4187-2_take_lid.jpg}
    \caption{\texttt{take\_lid}}
    \end{minipage}    
    &
    \begin{minipage}{.18\textwidth}
      \includegraphics[width=\linewidth, height=30mm]{images/base_w_teach_c_distil_w put-down_pan/4187-1_take_pan.jpg}
      \caption{\texttt{take\_pan}}
    \end{minipage}
    \\ \hline
    \multicolumn{5}{l}{\textbf{TARGET}: \texttt{put-down\_pan}} \\ \hline
    \multicolumn{5}{l}{\textbf{PREDICTIONS}} \\ 
    \multicolumn{5}{l}{\texttt{\textbf{AVT} : [put\_lid, stir\_pasta, put-down\_spoon, change\_temperature, stir\_pan]
}} \\ 
    \multicolumn{5}{l}{\texttt{\textbf{LM-teacher} : [\textcolor{red}{put-down\_pan}, wash\_pan, open\_door, take\_pan, dry\_saucepan]}} \\
    \multicolumn{5}{l}{\texttt{\textbf{AVT + LM teacher Distl}: [put\_lid, stir\_pasta, put-down\_spoon, change\_temperature,}}\\ 
    \multicolumn{5}{l}{open\_door]} \\\hline\hline    
  \end{tabular}}
  \caption{Figure 5: Example of instances where the base video-only model makes wrong prediction, the text-based teacher makes the correct prediction, however the teacher distilled video model makes incorrect prediction.}\label{fig:base_w_teacher_c_distil_w1}
  \end{figure*}
% ------------------------------------------------------------------
% Case: Base wrong, teacher correct, student wrong
% EXAMPLE 3 & 4
% ------------------------------------------------------------------ 
\captionsetup[figure]{labelformat=empty}
\begin{figure*}[!ht]
{
  \begin{tabular}{ m{2.8cm}  m{2.8cm}  m{2.8cm}  m{2.8cm}  m{2.8cm}  }
    \hline\hline
    % ------------------------------------------------------------
    % EXAMPLE-1
    % ------------------------------------------------------------
    \multicolumn{5}{c}{\textbf{EXAMPLE 3}} \\ \hline \hline
    \multicolumn{5}{l}{\textbf{INPUT}} \\
    \begin{minipage}{.18\textwidth}
      \includegraphics[width=\linewidth, height=30mm]{images/base_w_teach_c_distil_w_cut_onion/82-5_take_onion.jpg}
      \caption{\texttt{take\_onion}}
    \end{minipage}
    &
    \begin{minipage}{.18\textwidth}
     \includegraphics[width=\linewidth, height=30mm]{images/base_w_teach_c_distil_w_cut_onion/82-4_put-down_onion.jpg}
     \caption{\texttt{put-down\_onion}}
    \end{minipage}
    &
    \begin{minipage}{.18\textwidth}
      \includegraphics[width=\linewidth, height=30mm]{images/base_w_teach_c_distil_w_cut_onion/82-3_close_container.jpg}
      \caption{\texttt{close\_container}}
    \end{minipage}    
    &
    \begin{minipage}{.18\textwidth}
      \includegraphics[width=\linewidth, height=30mm]{images/base_w_teach_c_distil_w_cut_onion/82-2_take_spatula.jpg}
    \caption{\texttt{take\_spatula}}
    \end{minipage}    
    &
    \begin{minipage}{.18\textwidth}
      \includegraphics[width=\linewidth, height=30mm]{images/base_w_teach_c_distil_w_cut_onion/82-1_take_knife.jpg}
      \caption{\texttt{take\_knife}}
    \end{minipage}
    \\ \hline
    \multicolumn{5}{l}{\textbf{TARGET}: \texttt{cut\_onion}} \\ \hline
    \multicolumn{5}{l}{\textbf{PREDICTIONS}} \\ 
    \multicolumn{5}{l}{\texttt{\textbf{AVT}: [put\_container, take\_knife, turn-on\_tap, open\_fridge, put-down\_onion]
}} \\ 
    \multicolumn{5}{l}{\texttt{\textbf{LM-teacher}: [put-down\_knife, \textcolor{red}{cut\_onion}, mix\_food, open\_drawer, take\_spoon]}} \\
    \multicolumn{5}{l}{\texttt{\textbf{AVT + LM teacher Distl}: [put\_container, take\_knife, put-down\_knife, take\_container,}} \\
    \multicolumn{5}{l}{open\_fridge]} \\ \hline\hline
    % ------------------------------------------------------------
    % EXAMPLE-4
    % ------------------------------------------------------------
    \multicolumn{5}{c}{\textbf{EXAMPLE 4}} \\ \hline \hline
    \multicolumn{5}{l}{\textbf{INPUT}} \\
    \begin{minipage}{.18\textwidth}
      \includegraphics[width=\linewidth, height=30mm]{images/base_w_teach_c_distil_w_put-down_tomato/11144-5_take_dough.jpg}
      \caption{\texttt{take\_dough}}
    \end{minipage}
    &
    \begin{minipage}{.18\textwidth}
     \includegraphics[width=\linewidth, height=30mm]{images/base_w_teach_c_distil_w_put-down_tomato/11144-4_put_dough.jpg}
     \caption{\texttt{put\_dough}}
    \end{minipage}
    &
    \begin{minipage}{.18\textwidth}
      \includegraphics[width=\linewidth, height=30mm]{images/base_w_teach_c_distil_w_put-down_tomato/11144-3_put_lid.jpg}
      \caption{\texttt{put\_lid}}
    \end{minipage}    
    &
    \begin{minipage}{.18\textwidth}
      \includegraphics[width=\linewidth, height=30mm]{images/base_w_teach_c_distil_w_put-down_tomato/11144-2_open_door.jpg}
    \caption{\texttt{open\_door}}
    \end{minipage}    
    &
    \begin{minipage}{.18\textwidth}
      \includegraphics[width=\linewidth, height=30mm]{images/base_w_teach_c_distil_w_put-down_tomato/11144-1_take_tomato.jpg}
      \caption{\texttt{take\_tomato}}
    \end{minipage}
    \\ \hline
    \multicolumn{5}{l}{\textbf{TARGET}: \texttt{put-down\_tomato}} \\ \hline
    \multicolumn{5}{l}{\textbf{PREDICTIONS}} \\ 
    \multicolumn{5}{l}{\texttt{\textbf{AVT} : [open\_fridge, open\_door, turn-on\_tap, open\_drawer, rinse\_hand]}} \\ 
    \multicolumn{5}{l}{\texttt{\textbf{LM-teacher} : [\textcolor{red}{put-down\_tomato}, close\_door, take\_tomato, take\_plate, take\_pan]}} \\
    \multicolumn{5}{l}{\texttt{\textbf{AVT + LM teacher Distl}: [open\_fridge, open\_door, open\_drawer, close\_door,}} \\
    \multicolumn{5}{l}{take\_bowl]} \\\hline\hline    
  \end{tabular}}
  \caption{Figure 6: Example of instances where the base video-only model makes wrong prediction, the text-based teacher makes the correct prediction, however the teacher distilled video model makes incorrect prediction.}\label{fig:base_w_teacher_c_distil_w2}
\end{figure*}
